# Supplementary material for: MonoPair: Monocular 3D Object Detection Using Pairwise Spatial Relationships
Source: arXiv:2003.00504 source file (2020-03-01)
Supplement: Supplementary file 1 [file appendix.tex]

\section*{Appendix}

\begin{strip}\centering
	\vspace{-7cm}
		\centering

		\begin{tabular}{ c|c c c|c c c|c c c|c c c }
			\hline
			& \multicolumn{3}{c|}{$AP_{bv}$ IoU$\geq$0.5} & \multicolumn{3}{c|}{$AP_{3D}$ IoU$\geq$0.5} & \multicolumn{3}{c|}{$AP_{bv}$ IoU$\geq$0.7} & \multicolumn{3}{c}{$AP_{3D}$ IoU$\geq$0.7} \\
			\hline
			Methods  & E & M & H  & E & M & H  & E & M & H  & E & M & H \\
			
			\hline
			%xxx & - & - & - & - & - & - & - & - & - & - & - & - \\
			Mono3D \cite{chen_monocular_2016} & 30.50 & 22.34 & 19.16 & 25.19 & 18.20 & 15.52 & 5.22 & 5.19 & 4.13 & 2.53 & 2.31 & 2.31 \\ % IoU0.5 from ColorEmbed
			%CenterNet & 31.5$\pm$2.0 & 29.7$\pm$0.7 & 28.1$\pm$4.6 & - & - & - & - & - & - & - & - & - \\
			%CenterNet*	&34.04	&30.50	&26.78	&19.55	&18.62	&16.61	&3.54	&4.39	&3.57	&0.89	&1.15	&1.38 \\ % eval pretrain
			OFTNet \cite{roddick2018orthographic} & - & - & - & - & - & - & 11.06 & 8.79 & 8.91 & 4.07 & 3.27 & 3.29 \\ % from OFTNet
			MF3D \cite{xu_multilevel_2018} & 55.02 & 36.73 & 31.27 & 47.88 & 29.48 & 26.44 & 22.03 & 13.63 & 11.60 & 10.53 & 5.69 & 5.39 \\ %RT:120ms,from MonoPSR
			MonoPSR \cite{ku_monocular_2019} & 56.97 & 43.39 & 36.00 & 49.65 & 41.71 & 29.95 & 20.63 & 18.67 & 14.45 & 12.75 & 11.48 & 8.59 \\ %RT:200ms
			TLNet(mono) \cite{qin_triangulation_2019} & 52.72 & 37.22 & 32.16 & 48.34 & 33.98 & 28.67 & 21.91 & 15.72 & 14.32 & 13.77 & 9.72 & 9.29 \\
			MonoGRNet \cite{qin_monogrnet_2018}& 54.21 & 39.69 & 33.06 & 50.51 & 36.97 & 30.82 & 24.97 & 19.44 & 16.30 & 13.88 & 10.19 & 7.62 \\ % from TLNet
			%MonoGRNet*	&53.91	&39.45	&32.84	&50.27	&36.67	&30.53	&24.84	&19.27	&16.20	&13.84	&10.11	&7.59 \\ % eval results
			MonoDIS  \cite{simonelli_disentangling_2019}& - & - & - & - & - & - & 24.26 & 18.43 & 16.95 & 18.05 & 14.98 & 13.42  \\
			M3D-RPN \cite{brazil_m3d_rpn_2019}& 55.37 & 42.49 & 35.29 & 48.96 & 39.57 & 33.01 & 25.94 & 21.18 & 17.90 & 20.27 & 17.06 & 15.21 \\
			%M3D-RPN*	&55.37	&42.48	&35.29	&48.96	&39.57	&33.00	&25.94	&21.18	&17.90	&20.27	&17.05	&15.21 \\ % eval pretrain
			\hline
			Baseline & 54.50&	40.87&	34.45&	48.22&	36.80&	31.97&	25.69&	18.97&	16.48&	14.69&	10.27&	9.06 \\
			% +dv & 57.88	&47.11&	42.32&	53.77	&41.29&	39.01&	22.25&	18.78&	19.85&	17.66&	13.37&	15.27 \\
			$+\sigma^{z}+\sigma^{uv}$ & 58.49	 &48.57	 &43.20	 &54.68	 &42.43	 &40.17	 &26.22	 &21.09	 &19.78	 &19.27	 &16.57	 &14.50 \\
			MonoPair & \textbf{59.66} & \textbf{49.52} & \textbf{43.76} & \textbf{55.88} & \textbf{43.32} & \textbf{40.94} & \textbf{28.97} & \textbf{22.65} & \textbf{21.10} & \textbf{22.26} & \textbf{18.42} & \textbf{16.49} \\
			\hline
		\end{tabular}
    \vspace{7cm}
	\captionof{table}{$AP_{11}$ scores on KITTI3D validation set for car. E, M and H represent \textit{Easy}, \textit{Moderate} and \textit{Hard} samples.}
	\label{tab:ap11}
\end{strip}
\thispagestyle{empty}
\pagestyle{empty}

In the supplementary of MonoPair, we mainly show additional experimental results and comparisons with other methods.
A video, showing the sequential results of our method on the KITTI dataset, is uploaded in the supplementary directory as well.
The code and more high-resolution results of MonoPair can also be found in \url{https://sites.google.com/view/monopair}.

\subsection*{Additional Validation Results through $AP_{11}$}

As mentioned in the main paper, previous methods mainly conduct evaluation experiments through the old metric $AP_{11}$ on KITTI3D benchmark. 
Thus, To compare our method with more monocular 3D object detectors, we also show results on the KITTI3D validation set through $AP_{11}$ as shown in Table \ref{tab:ap11}. 
Our \textbf{Baseline}, as mentioned in the main paper, is mainly derived from CenterNet \cite{zhou_objects_2019}, which is designed specifically for 2D object detection.
It can not catch a similar performance as state-of-the-art monocular 3D object detectors. 
However, with the proposed uncertainty-aware spatial constraint optimization, our \textbf{MonoPair} finally outperforms all of the other methods with a large margin.
%Our method achieves the state-of-the-art result as well.

\subsection*{Additional Qualitative Results}
We also present additional qualitative results on KITTI validation set as shown in Figure \ref{fig:block}-\ref{fig:pedestrian}. 
We choose four different scenarios (block, town road, highway and city center), where two samples are selected from each of the scenarios.
Predictions from MonoGRNet \cite{qin_monogrnet_2018} and M3D-RPN \cite{brazil_m3d_rpn_2019}, and our MonoPair are presented in each figure from top to down.
Blue boxes mean predictions from cars. Yellow and gray boxes are predictions of pedestrians and cyclists respectively.
The cross shows the predicted orientation of the 3D object. More results are also uploaded in the supplementary directory.

Compared with results from other detectors as shown in these figures, MonoPair shows a great ability to detect seriously occluded samples. 
It also provides a considerable bounding box for samples far away from the camera. 
However, MonoGRBet \cite{qin_monogrnet_2018} and M3D-RPN \cite{brazil_m3d_rpn_2019} always neglect those occluded or further samples.
Besides, MonoPair also provides much better orientation predictions as shown in all the figures.
Figure \ref{fig:pedestrian} is mainly to show the detection ability for pedestrians and cyclists, which are trained from much fewer samples compared with cars.
The proposed spatial constraint from the same category provides more information for training and shows much accurate predictions.
\begin{figure*}[!t]
	\centering
	  \begin{subfigure}{0.65\linewidth}
		\includegraphics[width=\linewidth]{fig/supp/007256}
		\caption{}
		\label{fig:}
	\end{subfigure}
	\begin{subfigure}{0.65\linewidth}
		\includegraphics[width=\linewidth]{fig/supp/007350}
		\caption{}
		\label{fig:cons_key_view}
	\end{subfigure}
	\caption{Predictions on two block scenarios from the KITTI validation set. Results are from MonoGRNet \cite{qin_monogrnet_2018}, M3D-RPN \cite{brazil_m3d_rpn_2019}, and our MonoPair from top to down in both (a) and (b).}
	\label{fig:block}
\end{figure*}
\begin{figure*}[!t]
  \centering
  \begin{subfigure}{0.65\linewidth}
		\includegraphics[width=\linewidth]{fig/supp/007230}
		\caption{}
		\label{fig:cons_key_cam}
	\end{subfigure}
  \begin{subfigure}{0.65\linewidth}
		\includegraphics[width=\linewidth]{fig/supp/007266}
		\caption{}
		\label{fig:cons_key_view}
	\end{subfigure}
	\caption{Predictions on two town road scenarios from the KITTI validation set. Results are from MonoGRNet \cite{qin_monogrnet_2018}, M3D-RPN \cite{brazil_m3d_rpn_2019}, and our MonoPair from top to down in both (a) and (b).}
	\label{fig:townroad}
\end{figure*}
\begin{figure*}[!t]
  \centering
  \begin{subfigure}{0.65\linewidth}
		\includegraphics[width=\linewidth]{fig/supp/007352}
		\caption{}
		\label{fig:cons_key_cam}
	\end{subfigure}
  \begin{subfigure}{0.65\linewidth}
		\includegraphics[width=\linewidth]{fig/supp/007396}
		\caption{}
		\label{fig:cons_key_view}
	\end{subfigure}
	\caption{Predictions on two highway scenarios from the KITTI validation set. Results are from MonoGRNet \cite{qin_monogrnet_2018}, M3D-RPN \cite{brazil_m3d_rpn_2019}, and our MonoPair from top to down in both (a) and (b).}
	\label{fig:highway}
\end{figure*}
\begin{figure*}[!t]
  \centering
  \begin{subfigure}{0.65\linewidth}
		\includegraphics[width=\linewidth]{fig/supp/007202}
		\caption{}
		\label{fig:cons_key_view}
	\end{subfigure}
  \begin{subfigure}{0.65\linewidth}
		\includegraphics[width=\linewidth]{fig/supp/007318}
		\caption{}
		\label{fig:cons_key_view}
	\end{subfigure}
	\caption{Predictions on two city center scenarios especially for pedestrians and cyclists from the KITTI validation set. Results are from MonoGRNet \cite{qin_monogrnet_2018}, M3D-RPN \cite{brazil_m3d_rpn_2019}, and our MonoPair from top to down in both (a) and (b).}
	\label{fig:pedestrian}
\end{figure*}

%\section{Erratum}
%We are sorry for typing errors in the main file including
%\begin{itemize}
%	\item \textit{boundng} $\rightarrow$ \textit{bounding} in line 415,
%	\item \textit{showin} $\rightarrow$ \textit{shown} in line 514,
%	\item \textit{diagnal} $\rightarrow$ \textit{diagonal} in line 536,
%	\item \textit{dimesion} $\rightarrow$ \textit{dimension} in line 536,
%	\item \textit{varibles} $\rightarrow$ \textit{variables} in line 498 and line 548,
%	\item \textit{folloing} $\rightarrow$ \textit{following} in line 551,
%	\item \textit{pariwise} $\rightarrow$ \textit{pairwise} in line 572,
%	and \item \textit{ucertainty} $\rightarrow$ \textit{uncertainty} in line 783.
%\end{itemize}
%We will fix all of those errors in the updated version.
